# Supplementary material for: Flexible Integration of Gigahertz Nanomechanical Resonators with a Superconducting Microwave Resonator using a Bonded Flip-Chip Method
Source: arXiv:2304.13592 source file (2023-04-26)

(a)

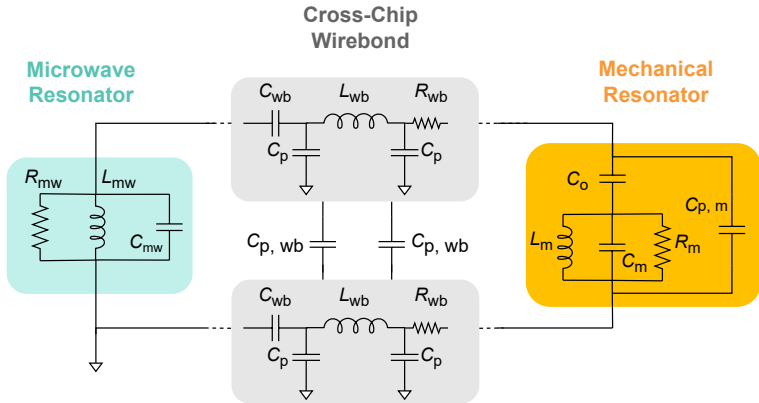

(b)

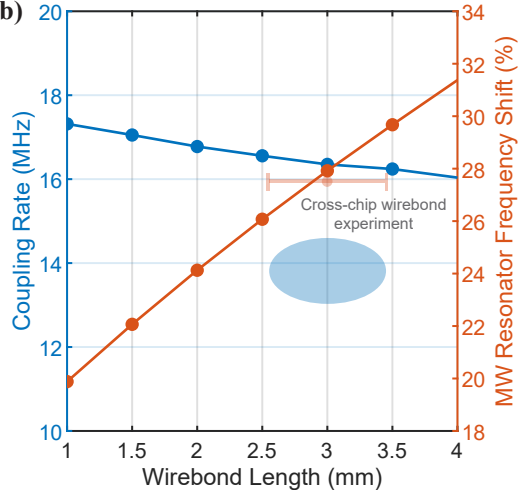

Supplement: Supplementary file 1 [file SI_Fig3_20221208.pdf]
