# Supplementary material for: Flexible Integration of Gigahertz Nanomechanical Resonators with a Superconducting Microwave Resonator using a Bonded Flip-Chip Method
Source: arXiv:2304.13592 source file (2023-04-26)

(a)

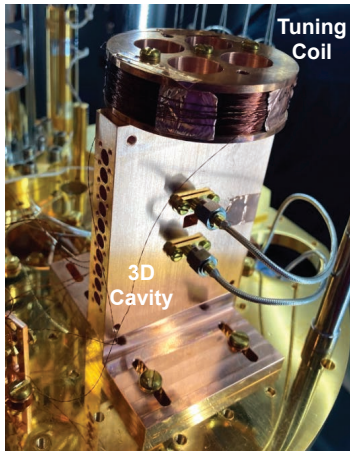

(b)

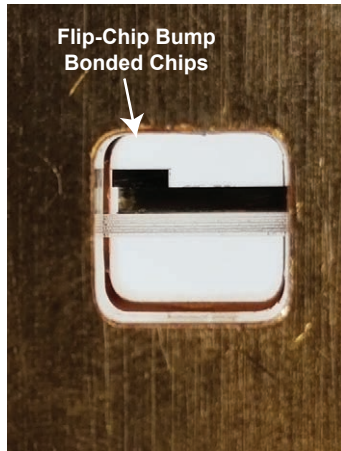

(c)

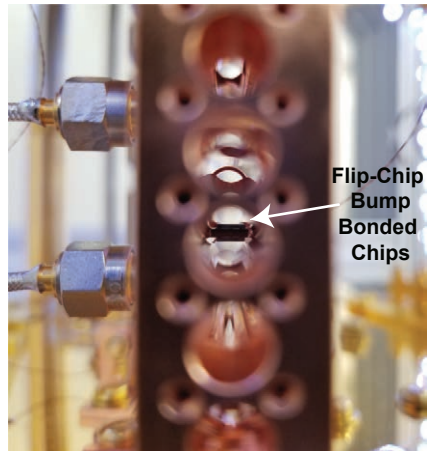

Supplement: Supplementary file 2 [file SI_Fig4_20221024.pdf]
